# Supplementary material for: Capillary force-driven particle orientation in rod networks
Source: arXiv:2503.18744 source file (2025-06-15)
Supplement: Supplementary file 1 [file SI.pdf]

1  
2  
3  
4  
5  
6  
7  
8  
9  
10  
11  
12  
13  
14  
15  
16  
17

**Supplementary Information**  
**for**  
**Capillary force-driven particle orientation in rod networks**

Lingyue Liu\*,<sup>1</sup> Sebastian Gassenmeier,<sup>1</sup> and Erin Koos\*<sup>1</sup>  
<sup>1</sup>*KU Leuven, Department of Chemical Engineering,  
Soft Matter, Rheology and Technology, 3001 Leuven, Belgium.*

**LIST OF FIGURES**

|    |                                                                                                                                      |   |
|----|--------------------------------------------------------------------------------------------------------------------------------------|---|
| S1 | Contact angle measurement of rod particles at bulk (black) and secondary liquid (yellow) interfaces. ....                            | 2 |
| S2 | Averaged side contact probability with different amounts of secondary liquids .....                                                  | 2 |
| S3 | Cross section of a liquid bridge between (a) two (b) three parallel rods in the central region. ....                                 | 3 |
| S4 | 3D reconstructed confocal micrographs of capillary suspension .....                                                                  | 3 |
| S5 | Polar angle probability as a function of particle position in capillary suspensions with different amounts of secondary liquid ..... | 4 |
| S6 | Schematic showing the clustering coefficient for various configurations of rods with a coordination number of 6 in 3D. ....          | 4 |

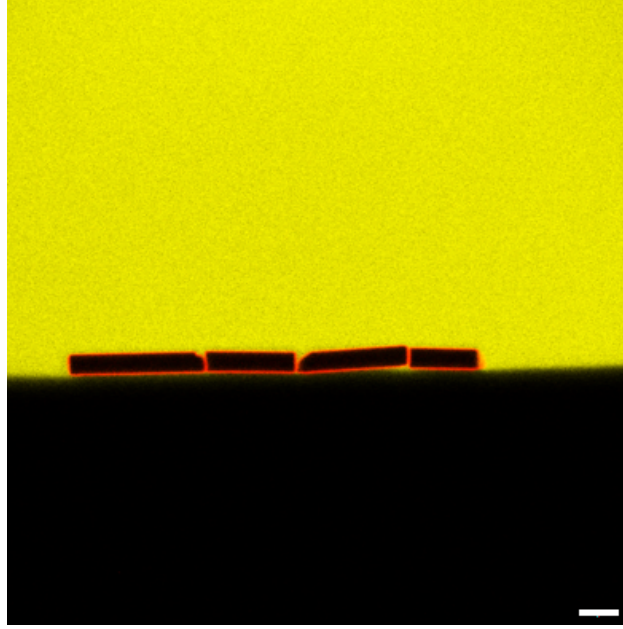

FIG. S1. Contact angle measurement of rod particles at bulk (black) and secondary liquid (yellow) interfaces. The scale bar is  $10\ \mu\text{m}$ .

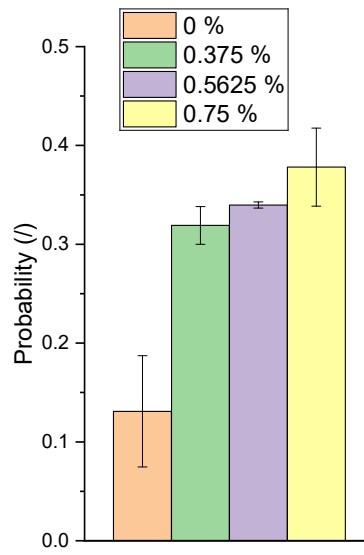

FIG. S2. Averaged side contact probability with different amounts of secondary liquids

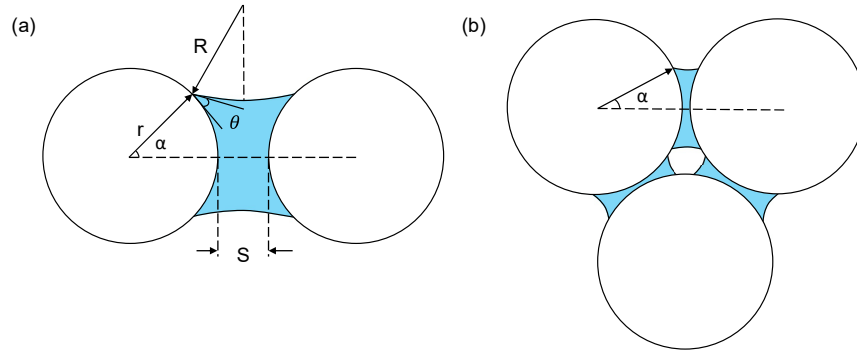

FIG. S3. Cross section of a liquid bridge between (a) two (b) three parallel rods in the central region.

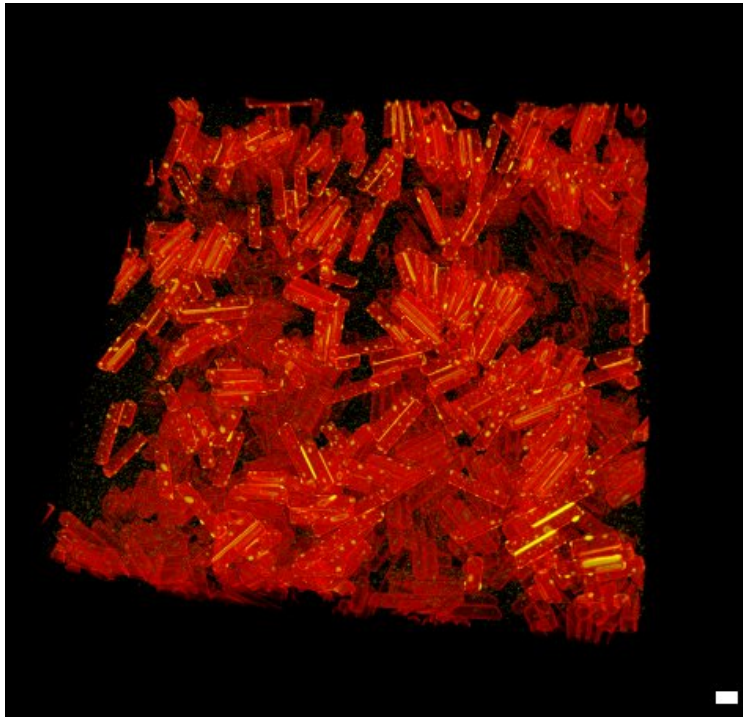

FIG. S4. 3D reconstructed confocal micrographs of capillary suspension with a secondary liquid of 0.75 % ( $\phi_{\text{sec}}/\phi_{\text{solid}} = 5\%$ ), the scale bar is 10  $\mu\text{m}$ .

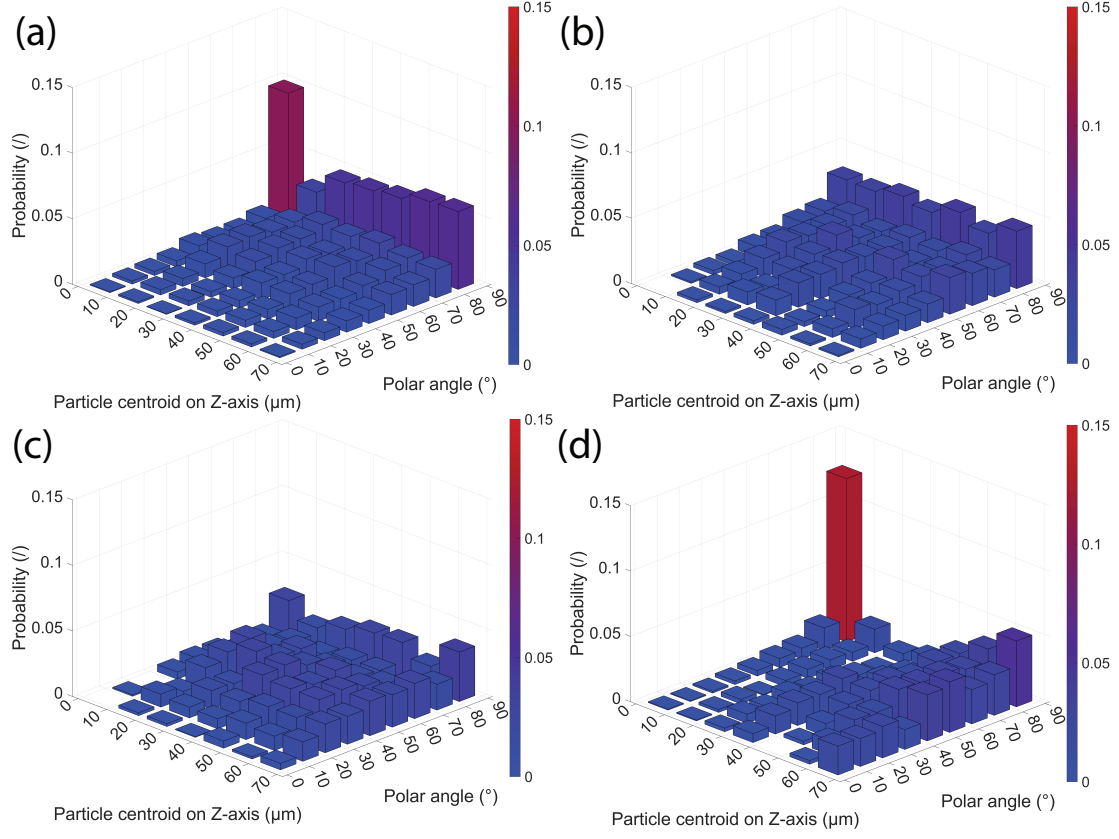

FIG. S5. Polar angle probability as a function of particle position in capillary suspensions with different amounts of secondary liquid (a) 0 % ( $\phi_{\text{sec}}/\phi_{\text{solid}} = 0.0$  %) (b) 0.375 % ( $\phi_{\text{sec}}/\phi_{\text{solid}} = 2.5$  %) (c) 0.5625 % ( $\phi_{\text{sec}}/\phi_{\text{solid}} = 3.75$  %) (d) 0.75 % ( $\phi_{\text{sec}}/\phi_{\text{solid}} = 5$  %).

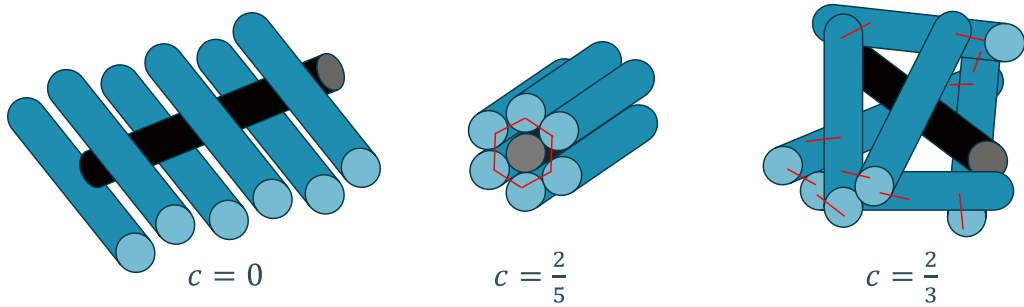

FIG. S6. Schematic showing the clustering coefficient for various configurations of rods with a coordination number of 6 in 3D.
